# Supplementary material for: RoboCraft: Learning to See, Simulate, and Shape Elasto-Plastic Objects with Graph Networks
Source: arXiv:2205.02909 source file (2022-05-05)
Supplement: Supplementary file 1 [file 060appendix.tex]

\section{Appendix}
\subsection{Hardware Specs}
\subsection{Visualized Target Shapes}
\subsection{Additional Results on Particle Sampling}
